# Supplementary material for: Classifier-independent Lower-Bounds for Adversarial Robustness
Source: arXiv:2006.09989 source file (2020-11-10)
Supplement: Supplementary file 1 [file supp_preamble.tex]

All through this supplemental and the main manuscript, $\mathcal X$ denotes the feature space.
% At times, this will be a metric space with metric denoted $d_{\mathcal X}$ or $d$ for short.
% The space of labels is $\mathcal Y = \{1,2\}$. There is a
The \emph{label (aka classification target)} is a random variable $Y$ with
values in $\mathcal Y = \{1,2\}$, and random variable $X$ called the
\textit{features}, with values in $\mathcal X$. We only consider binary
classification problems in this work. The goal is to predict $Y$ given $X$. This
corresponds to prescribing a measurable function $h:\mathcal X \rightarrow
\{1,2\}$, called a \emph{classifier}. Let $P$ be the (unknown) joint probability
distribution of $(X,Y)$. The goal of learning is to find a classifier $h$, such
that $h(X) = Y$ as often as possible, possibly under additional constraints.
% The presentation of more notation is deferred to section \ref{sec:bayesian} when we will have a genuine need for it.

\begin{mdframed}
{\bfseries General framework.} In this work, as in ~\cite{bhagoji2019}, we will
only consider binary classification problems under adversarial attacks, where
the labels are equiprobably , i.e $\mathbb P(Y=1)=\mathbb P(Y=2)=1/2$. These
assumptions are technical requirement needed to apply the Kantorovich-Rubinstein
duality formula of optimal-transport. Multiclass problems can be considered in one-versus-all fashion.
We will denote $P^k := \frac{1}{2}\mathbb P(X|Y=k)$ for $k=1,2$, so that the
classification problem is entirely captured by the pair $P=(P^1,P^2)$, called a
\emph{binary experiment}.
\end{mdframed}

\paragraph{Total-variation.} $\tv(Q,Q')$ denotes the total-variation distance between finite measures $Q$ and
$Q'$ on the same measurable space (typically the feature space , $\mathcal X$).

\input{adversarial_notations}
\input{transport.tex}
